# Supplementary material for: Study of Self-Interaction Errors in Density Functional Calculations of Magnetic Exchange Coupling Constants Using Three Self-Interaction Correction Methods
Source: arXiv:2205.05801 source file (2022-05-11)
Supplement: Supplementary file 1 [file SI.pdf]

# Supplemental Information for: Study of Self-Interaction Errors in Density-Functional Calculations of Magnetic Exchange Coupling Constants Using Three Self-Interaction-Correction Methods

Prakash Mishra,[†] Yoh Yamamoto,[‡] Po-Hao Chang,[‡] Duyen B. Nguyen,[¶] Juan E. Peralta,[¶] Tunna Baruah,[†,‡] and Rajendra R. Zope[*,†,‡]

†*Computational Science Program, University of Texas at El Paso, El Paso, Texas 79968, USA*

‡*Department of Physics, University of Texas at El Paso, El Paso, TX, 79968, USA*

¶*Physics Department and Science of Advanced Materials Program, Central Michigan University, Mt. Pleasant, Michigan 48859, USA*

E-mail: rzope@utep.edu

## $J_{SP}$ for H$\cdots$He multicenter systems

Let $E_{123}$ and $E_{1234}$ be the total energies of the system where the indices 1-4 are the spin state, either spin up ($\uparrow$) or spin down ($\downarrow$), at the site labeled accordingly as Fig. S1. Then, the spin projected coupling constants $J_{SP}$ of the four H$\cdots$He systems are written as follows.

- $H_3He_2$

$$E_{\downarrow\uparrow\downarrow} - E_{\uparrow\uparrow\uparrow} = J_{12}$$

$$2(E_{\uparrow\uparrow\downarrow} - E_{\uparrow\uparrow\uparrow}) = J_{12} + J_{13}$$

- $H_4He_3$

$$\begin{aligned}
E_{\uparrow\downarrow\downarrow\uparrow} - E_{\uparrow\uparrow\uparrow\uparrow} &= J_{12} + J_{13} \\
E_{\uparrow\downarrow\uparrow\downarrow} - E_{\uparrow\uparrow\downarrow\downarrow} &= J_{12} - J_{13} \\
E_{\uparrow\downarrow\uparrow\downarrow} - E_{\uparrow\uparrow\uparrow\uparrow} &= J_{12} + \frac{1}{2}J_{13} + \frac{1}{2}J_{14} \\
E_{\uparrow\uparrow\downarrow\downarrow} - E_{\uparrow\downarrow\downarrow\uparrow} &= -J_{12} + \frac{1}{2}J_{13} + \frac{1}{2}J_{14}
\end{aligned}$$

where we neglect the $J_{14}$ term.

- $H_3He_3$

$$E_{\downarrow\uparrow\uparrow} - E_{\uparrow\uparrow\uparrow} = J_{12}$$

- $H_4He_4$

$$E_{\downarrow\uparrow\downarrow\uparrow} - E_{\uparrow\uparrow\uparrow\uparrow} = 2J_{12}$$

$$E_{\uparrow\uparrow\downarrow\downarrow} - E_{\uparrow\uparrow\uparrow\uparrow} = J_{12} + J_{13}$$

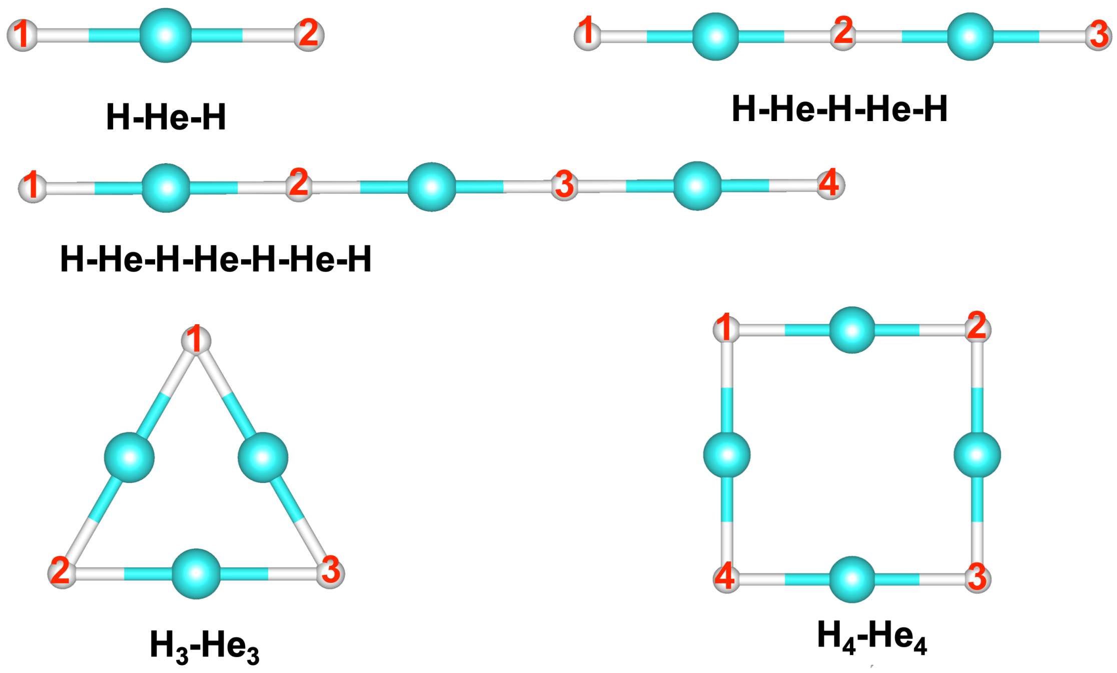


Figure S1: H$\cdots$He multicenter systems where the spin centers are labeled with numbers in red color.
